# Supplementary material for: ML$^2$Tuner: Efficient Code Tuning via Multi-Level Machine Learning Models
Source: arXiv:2411.10764 source file (2024-11-16)
Supplement: Supplementary file 1 [file 41_Appendix_Model.tex]

%  \begin{table}
%   \caption{Profiling Layer of Convolution in ResNet18~\cite{resnet18}}
%   \centering
%   \label{tab:resnet18_architecture}
%   \begin{tabular}{llllll}
%     \toprule
%     Index & Name & H,W,C & KN,KH,KW & P,S & OH,OW \\
%     \midrule
%     1 & Conv 0-3 & 56,56,64 & 64,3,3 & 1,1 & 56,56 \\ 
%     2 & Conv 4 & 56,56,64 & 128,1,1 & 0,2 & 28,28 \\ 
%     3 & Conv 5 & 56,56,64 & 128,3,3 & 1,2 & 28,28 \\ 
%     4 & Conv 6-8 & 28,28,128 & 128,3,3 & 1,1 & 28,28 \\ 
%     5 & Conv 9 & 28,28,128 & 256,1,1 & 0,2 & 14,14 \\ 
%     6 & Conv 10 & 56,56,64 & 128,1,1 & 0,2 & 28,28 \\ 
%     7 & Conv 11-13 & 56,56,64 & 128,3,3 & 1,2 & 28,28 \\ 
%     8 & Conv 14 & 28,28,128 & 128,3,3 & 1,1 & 28,28 \\
%     9 & Conv 15 & 56,56,64 & 128,3,3 & 1,2 & 28,28 \\ 
%     10 & Conv 16-18 & 28,28,128 & 128,3,3 & 1,1 & 28,28 \\
%     \bottomrule
%   \end{tabular}
% \end{table}
