# Supplementary material for: ML$^2$Tuner: Efficient Code Tuning via Multi-Level Machine Learning Models
Source: arXiv:2411.10764 source file (2024-11-16)
Supplement: Supplementary file 2 [file 43_X_Appendix_HyperParameter.tex]

% %%% Hyper Paramerter

% \section{Experimental Parameter}


% \begin{table}[h!]
% \centering
% \caption{Ratio of configuration}
% \begin{tabular}{cccc}
% \toprule
% \textbf{Name} & \textbf{Valid} & \textbf{Number} & $\frac{\textbf{Valid}}{\textbf{Number}}$ \\
% \midrule
% Conv 1 & 4356 & 25088 & 0.1736 \\
% Conv 2 & 5104 & 25088 & 0.2034 \\ 
% Conv 3 & 4874 & 25088 & 0.1943 \\ 
% Conv 4 & 7689 & 25088 & 0.3065 \\ 
% Conv 5 & 11920 & 25088 & 0.4751 \\
% Conv 6 & 11920 & 25088 & 0.4751 \\
% Conv 7 & 11920 & 25088 & 0.4751 \\
% Conv 8 & 12400 & 25088 & 0.4943 \\
% Conv 9 & 12400 & 25088 & 0.4943 \\
% Conv 10 & 12400 & 25088 & 0.4943 \\
% \bottomrule
% \end{tabular}

% \end{table}

% %%%%%


% \begin{table}[h]
% \centering
% \label{tab:hyper_parameter_with_resnet18}
% \caption{Hyperparameters for Exploring the Optimal Task on \systemName}
% \begin{tabular}{lccc}
% \toprule
% \multicolumn{1}{c}{\textbf{Parameter}}       & \textbf{ML Model P}  & \textbf{ML Model V} & \textbf{ML Model A} \\ \midrule
% objective        & reg:squarederror             & binary:hinge             & reg:squarederror             \\ 
% max\_depth       & 14                        & 5                        & 14                        \\ 
% min\_child\_weight & 3                      & 3                        & 3                        \\ 
% gamma            & 0.0                        & 0.0                        & 0.0                      \\ 
% learning rate              & 0.01                      & 0.1                      & 0.01                      \\ 
% subsample        & 1.0                      & 0.6                      & 1.0                      \\ 
% colsample\_bytree & 1.0                     & 0.6                      & 1.0                      \\ 
% reg\_alpha       & 1e-2                     & 1e-5                     & 1e-05                    \\ 
% % learning rate == eta ...
% % learning\_rate   & 0.01                      & 0.1                      & 0.01                    \\ 
% \bottomrule
% \end{tabular}
% \end{table}

% \begin{table}[h]
% \centering
% \label{tab:range_parameter_tuning}
% \caption{Exploration Range for Optimal Hyperparameter Tuning}
% \begin{tabular}{lccc}
% \toprule
% \multicolumn{1}{c}{\textbf{Parameter}}       & \textbf{Search Sapce} & \textbf{Step} & \textbf{Available Space}
% \\ \midrule
% max depth & [3, 15] & 1 & [0, $\infty$] \\ 
% min child weight & [1, 10) & 1 & [0, $\infty$] \\
% gamma & [0.0, 1) & 0.1 & [0, $\infty$] \\
% subsample & [0.4, 1.0] & 0.1 & (0, 1] \\
% colsample bytree & [0.5, 1.0] & 0.1 & [0, 1] \\ 
% \midrule
% \multicolumn{1}{c}{\textbf{Parameter}}       & \multicolumn{2}{c}{\textbf{Search Sapce}} & \textbf{Available Space} \\
% \midrule
% % eta & \multicolumn{2}{c}{0.005, 0.01, 0.05, 0.1, 0.2, 0.3}  & [0, 1] \\
% reg alpha & \multicolumn{2}{c}{1e\{-5, -2, -1, 0, 1\}}  &  [0, $\infty$] \\
% % learning rate는 eta의 alias임.
% learning rate & \multicolumn{2}{c}{0.001, 0.01, 0.1, 0.2, 0.3} & [0, 1] \\

% \bottomrule 
% \end{tabular}
% \end{table}
% % 56 - (nTileW - 1) * 1
% % OW - (nTileW * TW) + TW

% % \begin{table}[h]
% % \centering
% % \label{tab:feature_in_task_on_evta}
% % \caption{Task에 구성되어 있는 Feature의 요소}
% % \begin{tabular}{llll}
% % \toprule
% % \multicolumn{1}{c}{Kernel Feature} & \multicolumn{1}{c}{Description} & \multicolumn{1}{c}{Hidden Feature} & \multicolumn{1}{c}{Description} \\
% % \midrule
% % IN     & Number of Input   & sizeOutTileW & TW \\
% % IH     & Height of Input   & sizeOutTileH & TH \\
% % IW     & Width of Input   & sizeInTileW & $(TW - 1) \times stride + KW$ \\
% % IC     & Channel of Input   & sizeInTileH & $(TH - 1) \times stride + KH$ \\
% % KN    & Number of Kernel Filter  & nTileW & $\left\lceil\frac{\text{OW}}{\text{TW}}\right\rceil$ \\
% % KH    & Height of Kernel Filter   & nTileH & $\left\lceil\frac{\text{OH}}{\text{TH}}\right\rceil$ \\
% % KW    & Width of Kernel Filter   & sizeOutTileBoundaryW & $OW - nTileW * TW$  \\
% % pad   & Padding & nFilterInLoop & TBD \\
% % stride & Stride   & InLoopOfnFilterInLoop & TBD \\
% % doReLu  & Fused Activation 연산인가?   & outDummyH &  \\
% % doBias & Bias 연산이 포함되어 있는가?   &  reSizedOutTileH & 
% %  \\
% % Shift & 양자화된 Scale 정보 $\frac{\text{$Scale_{in}$} \times \text{$Scale_{filter}$}}{\text{$Scale_{out}$}}$ & reSizedInTileH &  \\
% % OH  & Height of Output   & nVirtualThread & TBD \\
% % OW  & Width of Output   &  \\
% % nVT   & Num of Virtual Thread   &  \\
% % TH    & Tile Height Size   &  \\
% % TW    & Tile Width Size   &       &  \\
% % \bottomrule
% % \end{tabular}
% % \end{table}
